# Supplementary material for: Collaborative Inference for Large Models with Task Offloading and Early Exiting
Source: arXiv:2412.08284 source file (2024-12-11)
Supplement: Supplementary file 1 [file appendix.tex]

%\newpage

\appendices

\section{Proof of theorem 1} \label{appen:proof_theorem_1}

\begin{IEEEproof}
	% \rednote{Due to the smoothness in Assumption \ref{Lip}, taking expectation of $F\left(\boldsymbol{w}^{h+1}\right)$ and $F\left(\boldsymbol{w}^{h}\right)$
	% over the randomness in the $h$-th epoch, then proceeding to use Lemma \ref{lemma1}, Lemma \ref{lemma2} and Lemma \ref{lemma3}, we have}
	% Due to the smoothness in Assumption \ref{Lip} on global loss function,
	% %by using unbiased estimate stochastic 
	% by using the gradient $\mathbf{g}^{h}$ in Eq. \eqref{equ:gradient}, we have
	According to the smoothness property in Assumption \ref{Lip} and the definition of stochastic gradient $\mathbf{g}^{h}$ in Eq. \eqref{equ:gradient},
	we have:
	\begin{equation}
	%    \begin{small}
		\begin{aligned}
		\notag&F(\boldsymbol{w}^{h+1})-F(\boldsymbol{w}^{h})
		\leq -\alpha \left\langle\nabla F(\boldsymbol{w}^{h}), \mathbf{g}^{h}\right\rangle +\frac{\alpha^{2} L}{2} \|\mathbf{g}^{h}\|^{2}
		\end{aligned}
	%    \end{small}
	\end{equation}
	After applying the model compression technique with $\operatorname{top}_{k}$ operator, the expectation of the above inequality is expressed as:
	\begin{equation}
		%    \begin{small}
		\begin{aligned}
		\notag&\mathbb{E}\left[\mathbb{E}_{\operatorname{top}_{k}}\left[F(\boldsymbol{w}^{h+1})-F(\boldsymbol{w}^{h})\right]\right] \\
		&\leq -\alpha \mathbb{E}\left[\left\langle\nabla F(\boldsymbol{w}^{h}), \mathbf{g}^{h}\right\rangle\right]+\frac{\alpha^{2} L}{2} \mathbb{E}\left[\mathbb{E}_{\operatorname{top}_{k}}\left[\|\mathbf{g}^{h}\|^{2}\right]\right]
		\end{aligned}
		%    \end{small}
	\end{equation}
	For the sake of expression, we use $\mathbb{E}_{\operatorname{top}_{k}}\left[\nabla F(\boldsymbol{w}^{h})\right]$ to denote $\mathbb{E}\left[\nabla F\left( \operatorname{top}_{k} (\boldsymbol{w}^{h})\right)\right]$.
	We proceed to use Lemmas \ref{lemma1}-\ref{lemma3} to bound right hand side of the inequality, and obtain:
	\begin{equation}
	%    \begin{small}
	\begin{aligned}
	\notag&\mathbb{E}\left[\mathbb{E}_{\operatorname{top}_{k}}\left[F(\boldsymbol{w}^{h+1})-F(\boldsymbol{w}^{h})\right]\right] \\
	&\leq \frac{\alpha \eta}{2 N}\sum_{i=1}^{N} \sum_{k=0}^{\tau-1} \left[-\|\nabla F(\boldsymbol{w}^{h})\|^{2}-\|\mathbf{g}_{i}^{(k, h)}\|^{2}\right]\\
	&+\frac{\alpha \eta}{2 N} \sum_{i=1}^{N} \sum_{k=0}^{\tau-1} \left[L^{2} \eta^{2} \sum_{c=0}^{\tau-1}\left[\tau\|\mathbf{g}_{i}^{(k, h)}\|^{2}+\sigma^{2}\right]\right]\\
	&+\frac{(2-\gamma) \alpha^{2} L}{2}\left[\frac{\eta^{2} \tau}{N} \sum_{i=1}^{N} \sum_{k=0}^{\tau-1}\|\mathbf{g}_{i}^{(k, h)}\|^{2}+\frac{\tau \eta^{2} \sigma^{2}}{N}\right] \\
	&\stackrel{\circled{1}}{\leq} \frac{\alpha \eta}{2 N} \sum_{i=1}^{N} \sum_{k=0}^{\tau-1}\left[-\|\nabla F(\boldsymbol{w}^{h})\|^{2}-\|\mathbf{g}_{i}^{(k, h)}\|^{2}\right]\\
	&+\frac{\alpha \eta}{2 N}\sum_{i=1}^{N} \sum_{k=0}^{\tau-1}\left[\tau L^{2} \eta^{2}\left[\tau\|\mathbf{g}_{i}^{(k, h)}\|^{2}+\sigma^{2}\right]\right] \\
	&+\frac{(2-\gamma) \alpha^{2} L}{2}\left[\frac{\eta^{2} \tau}{N} \sum_{i=1}^{N} \sum_{k=0}^{\tau-1}\|\mathbf{g}_{i}^{(k, h)}\|^{2}+\frac{\tau \eta^{2} \sigma^{2}}{N}\right] \\
	&=-\eta \alpha \frac{\tau}{2}\|\nabla F(\boldsymbol{w}^{h})\|^{2} \\
	&-\left(1-\tau^2 L^{2} \eta^{2} -(2-\gamma) \eta \alpha L \tau\right) \frac{\eta \gamma}{2 N} \sum_{i=1}^{N} \sum_{k=0}^{\tau-1}\|\mathbf{g}_{i}^{(k, h)}\|^{2}\\
	&+\frac{L \tau \alpha \eta^{2}}{2 N}\left(N L \tau \eta+\alpha(2-\gamma)\right) \sigma^{2} \\
	&\stackrel{\circled{2}}{\leq}-\eta \alpha \frac{\tau}{2}\|\nabla F(\boldsymbol{w}^{h})\|^{2}+\frac{L \tau \alpha \eta^{2}}{2 N}\left(N L \tau \eta+\alpha(2-\gamma)\right) \sigma^{2}
	\end{aligned}
	%    \end{small}
	\end{equation}
	where in $\circled{1}$ we incorporate outer summation $\sum_{k=0}^{\tau-1}$, and $\circled{2}$ follows from Eq. (\ref{condtion1}).
	% \begin{equation}
	%     \tau^{2} L^{2} \eta^{2}+\left(2-\gamma\right) \eta \alpha L \tau \le 1
	% \end{equation}
	Finally, when summing up for all $H$ communication rounds and rearranging the terms, we can get Eq. \eqref{convergance1}, and the proof is completed.
	\end{IEEEproof}
